# Supplementary material for: Multi-criteria Token Fusion with One-step-ahead Attention for Efficient Vision Transformers
Source: arXiv:2403.10030 source file (2024-04-01)
Supplement: Supplementary file 4 [file figure_s1.tex]

 % \begin{figure}[h]
 %    \centering
 %    \begin{subfigure}{0.48\linewidth}
 %      \centering
 %       \includegraphics[trim=0 0 0 0,clip,width=\textwidth]{Figures/informative1.png}
 %      \caption{\textbf{Information loss.}}
 %      \label{fig:il_1}
 %    \end{subfigure}
 %    \hfill
 %    \begin{subfigure}{0.48\linewidth}
 %      \centering
 %       \includegraphics[trim=0 0 0 0,clip,width=\textwidth]{Figures/informative2.png}
 %      \caption{\textbf{The ratio of the information loss.}}
 %      \label{fig:il_2}
 %    \end{subfigure}

 % \end{figure}

 \begin{figure}[t!]
    \centering
       \includegraphics[trim=0 0 0 0,clip,height=0.95\textheight]{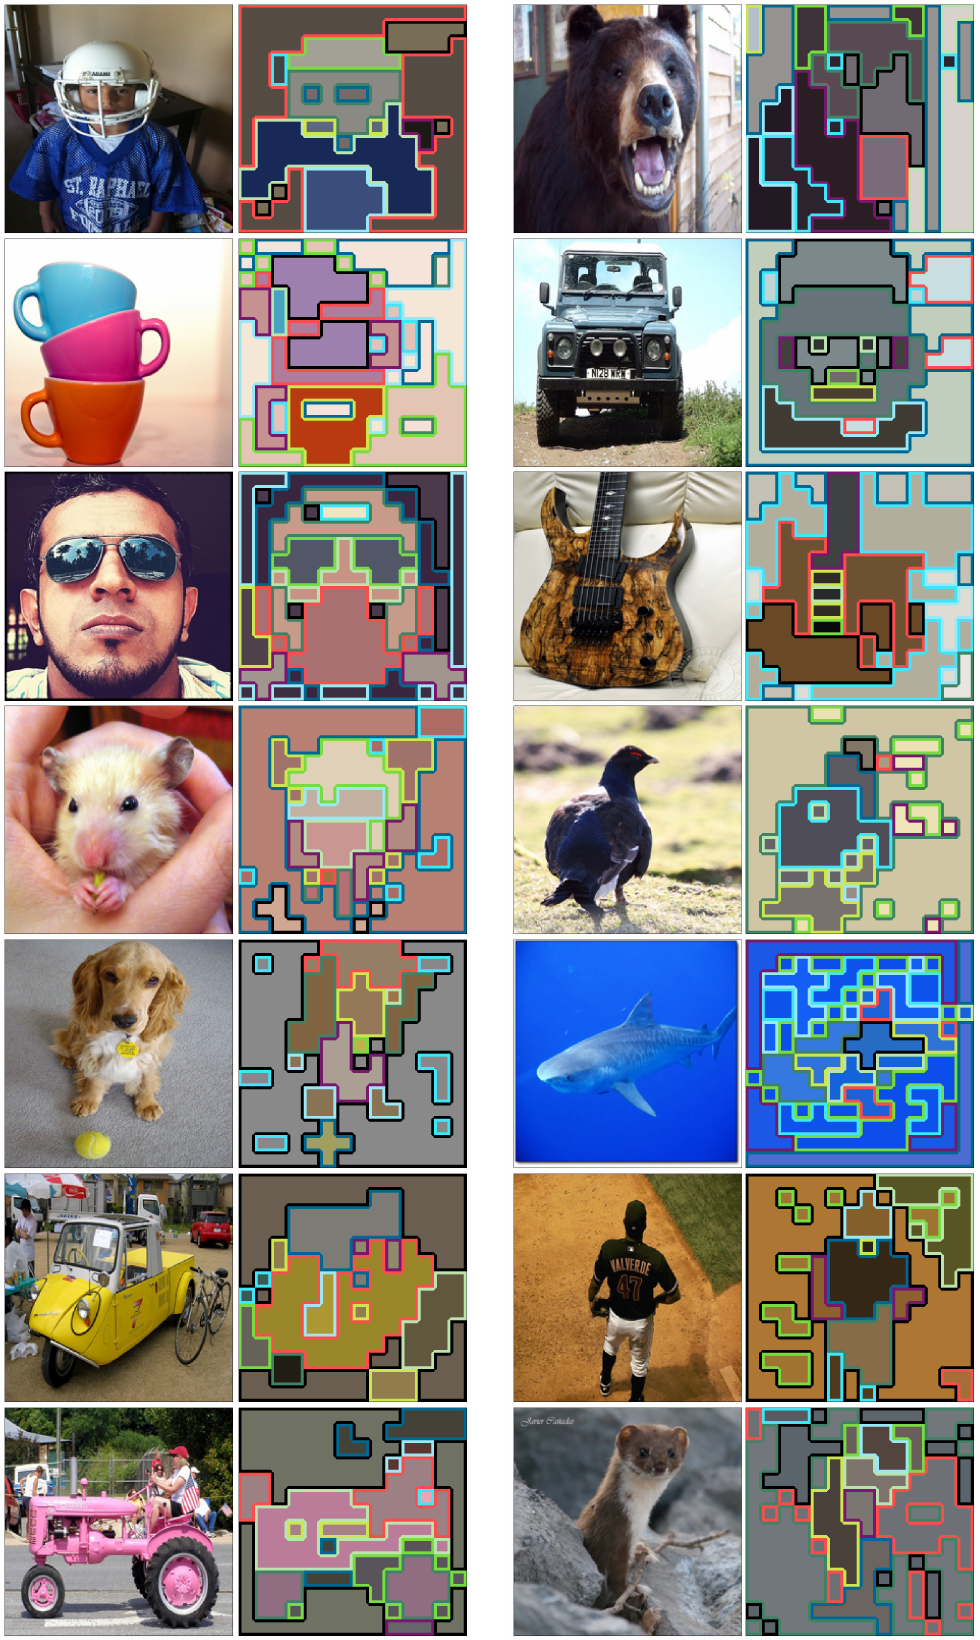}
      \caption{\textbf{Visualization of fused tokens.}}
      \label{fig:vis1}
 \end{figure}

 \begin{figure}[t!]
    \centering
       \includegraphics[trim=0 0 0 0,clip,height=0.95\textheight]{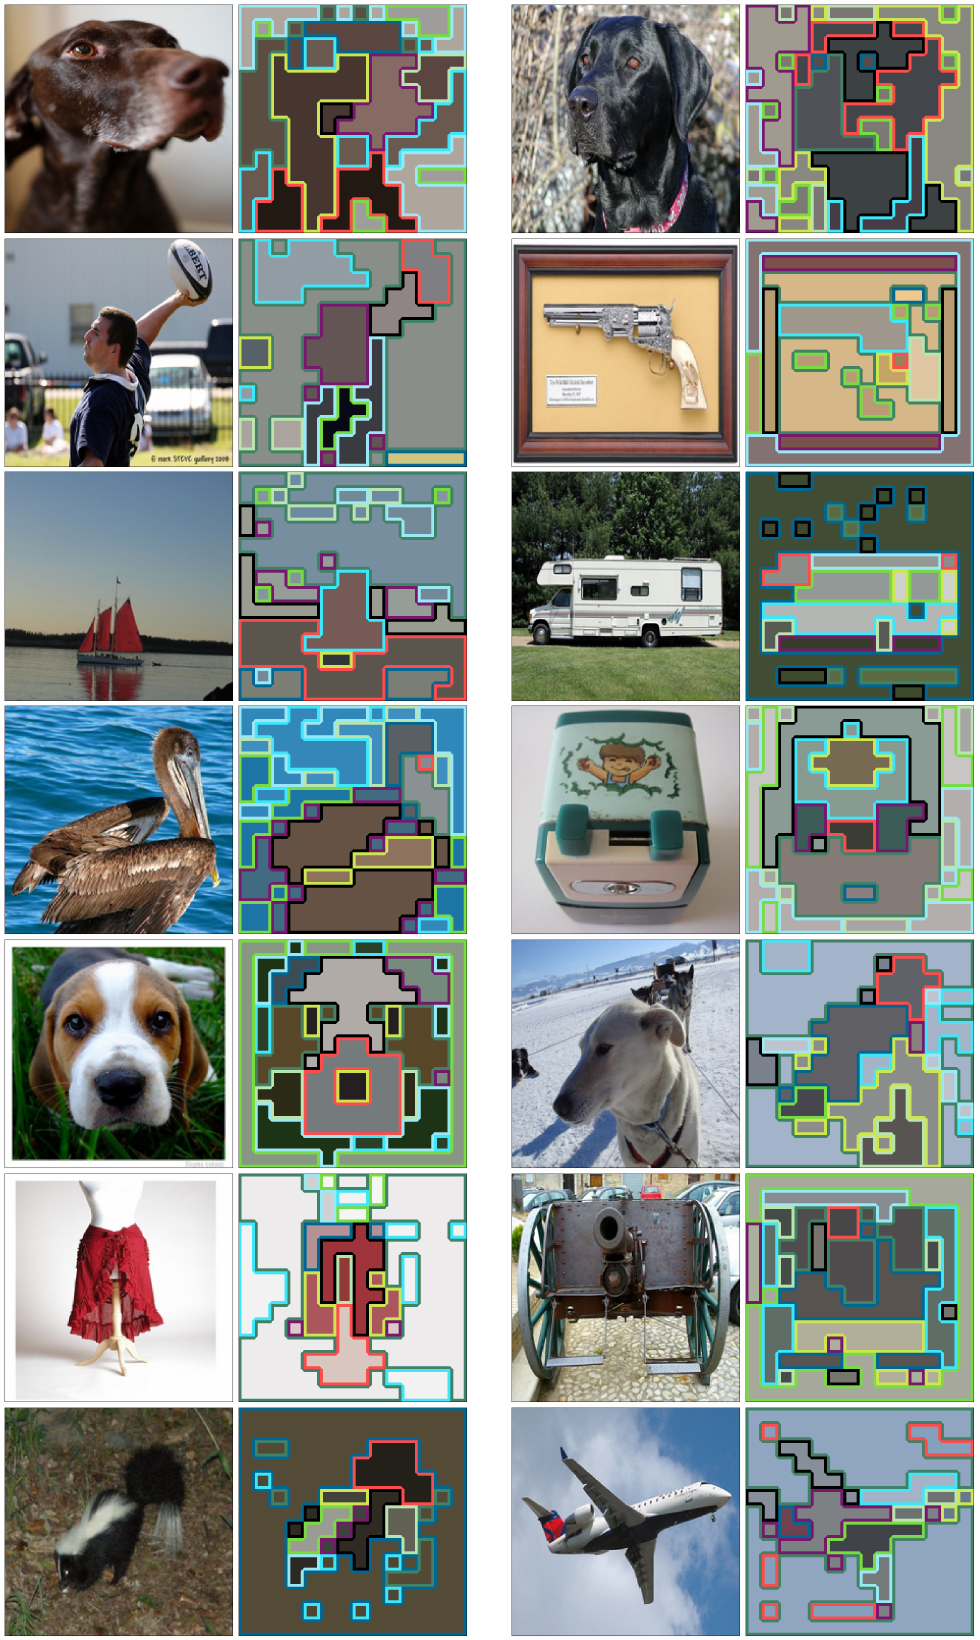}
      \caption{\textbf{Visualization of fused tokens.}}
      \label{fig:vis2}
 \end{figure}
