# Supplementary material for: Multi-criteria Token Fusion with One-step-ahead Attention for Efficient Vision Transformers
Source: arXiv:2403.10030 source file (2024-04-01)
Supplement: Supplementary file 6 [file table_s1.tex]

\begin{table}[h]
  \centering 
  \caption{\textbf{Detailed results after finetuning with $r=16$.}}
  \label{tab:sup1} 
  \setlength{\tabcolsep}{8pt}
  \begin{tabular}{c|ccc|ccc|ccc}
  \toprule
  \multicolumn{1}{c|}{\multirow{3}{*}{$r$}}  &\multicolumn{3}{c|}{DeiT-T}& \multicolumn{3}{c|}{DeiT-S}& \multicolumn{3}{c}{DeiT-B}\\
\multicolumn{1}{c|}{} & FLOPs & thr. & acc & FLOPs & thr. & acc.  & FLOPs & thr. & acc.\\
  \midrule
  %DeiT-T~\cite{touvron2021training}      &      &    3181  & 72.2      \\ 
     \rowcolor{Gray} Base & 1.26 & 3181 & 72.2 & 4.61 & 1262 & 79.8 & 17.58 & 412 & 81.8\\
     \midrule

     % 0  &  1.3  &  3154  &  73.0  &   4.6  &  1209  &  79.9  &  17.6  &  398  &  82.1 \\
     1  &  1.24  &  2829  &  73.0  & 4.51  &  1143  &  79.9  &  17.16  &  389  &  82.0 \\
     2  &  1.20  &  2904  &  73.0  & 4.38  &  1174  &  79.9  &  16.65  &  401  &  82.0 \\
     3  &  1.16  &  2995  &  73.0  & 4.24  &  1211  &  79.9  &  16.14  &  415  &  82.0 \\
     4  &  1.12  &  3084  &  73.0  & 4.10  &  1249  &  80.0  &  15.64  &  427  &  82.0 \\
     5  &  1.08  &  3188  &  73.0  & 3.97  &  1289  &  80.0  &  15.13  &  442  &  82.0 \\
     6  &  1.05  &  3296  &  72.9  & 3.83  &  1333  &  79.9  &  14.63  &  457  &  81.9 \\
     7  &  1.01  &  3441  &  72.9  & 3.70  &  1391  &  79.9  &  14.13  &  475  &  81.8 \\
     8  &  0.97  &  3579  &  72.8  & 3.56  &  1445  &  79.8  &  13.63  &  494  &  81.9 \\
     9  &  0.93  &  3719  &  72.8  & 3.43  &  1507  &  79.9  &  13.13  &  510  &  81.9 \\
    10  &  0.90  &  3879  &  72.8  & 3.30  &  1572  &  79.8  &  12.63  &  534  &  81.8 \\
    11  &  0.86  &  4022  &  72.8  & 3.17  &  1635  &  79.8  &  12.14  &  557  &  81.8 \\
    12  &  0.83  &  4200  &  72.7  & 3.04  &  1704  &  79.9  &  11.65  &  578  &  81.8 \\
    13  &  0.79  &  4376  &  72.8  & 2.91  &  1777  &  79.8  &  11.16  &  605  &  81.7 \\
    14  &  0.76  &  4565  &  72.8  & 2.79  &  1858  &  79.8  &  10.67  &  646  &  81.7 \\
    15  &  0.72  &  4775  &  72.7  & 2.66  &  1940  &  79.8  &  10.18  &  663  &  81.5 \\
    16  &  0.69  &  4992  &  72.6  & 2.53  &  2016  &  79.9  &   9.60  &  695  &  81.3 \\

  \bottomrule
  \end{tabular}
\end{table}
