# Supplementary material for: Multi-criteria Token Fusion with One-step-ahead Attention for Efficient Vision Transformers
Source: arXiv:2403.10030 source file (2024-04-01)
Supplement: Supplementary file 7 [file table_s2.tex]

\begin{table}[h]
  \centering 
  \caption{\textbf{Detailed results without training.}}
  \label{tab:sup2} 
  \setlength{\tabcolsep}{8pt}
  \begin{tabular}{c|ccc|ccc|ccc}
  \toprule
  \multicolumn{1}{c|}{\multirow{3}{*}{$r$}}  &\multicolumn{3}{c|}{DeiT-T}& \multicolumn{3}{c|}{DeiT-S}& \multicolumn{3}{c}{DeiT-B}\\
\multicolumn{1}{c|}{} & FLOPs & thr. & acc & FLOPs & thr. & acc.  & FLOPs & thr. & acc.\\
  \midrule
  %DeiT-T~\cite{touvron2021training}      &      &    3181  & 72.2      \\ 
     \rowcolor{Gray}Base  & 1.26 & 3181 & 72.2 & 4.61 & 1262 & 79.8  & 17.58 & 412 & 81.8  \\
     % 0  &  1.3  &  3133  &  72.1  &  4.6  &  1223  &  79.8  &  17.6  &  394  &  81.8 \\
     1  &  1.24  &  2795  &  72.1  &  4.51  &  1153  &  79.8  &  17.16  &  386  &  81.8 \\
     2  &  1.20  &  2868  &  72.1  &  4.38  &  1186  &  79.8  &  16.65  &  398  &  81.7 \\
     3  &  1.16  &  2972  &  72.1  &  4.24  &  1224  &  79.8  &  16.14  &  412  &  81.7 \\
     4  &  1.12  &  3061  &  72.1  &  4.10  &  1263  &  79.8  &  15.64  &  424  &  81.8 \\
     5  &  1.08  &  3168  &  72.1  &  3.97  &  1305  &  79.7  &  15.13  &  438  &  81.8 \\
     6  &  1.05  &  3275  &  72.0  &  3.83  &  1347  &  79.7  &  14.63  &  453  &  81.6 \\
     7  &  1.01  &  3418  &  71.9  &  3.70  &  1406  &  79.7  &  14.13  &  471  &  81.5 \\
     8  &  0.97  &  3545  &  71.9  &  3.56  &  1458  &  79.7  &  13.63  &  489  &  81.5 \\
     9  &  0.93  &  3699  &  71.8  &  3.43  &  1516  &  79.6  &  13.13  &  507  &  81.3 \\
    10  &  0.90   &  3842  &  71.7  &  3.30  &  1583  &  79.6  &  12.63  &  530  &  81.3 \\
    11  &  0.86  &  3995  &  71.7  &  3.17  &  1646  &  79.5  &  12.14  &  552  &  81.2 \\
    12  &  0.83  &  4160  &  71.7  &  3.04  &  1720  &  79.4  &  11.65  &  574  &  81.0 \\
    13  &  0.79  &  4346  &  71.5  &  2.91  &  1792  &  79.5  &  11.16  &  600  &  80.8 \\
    14  &  0.76  &  4527  &  71.3  &  2.79  &  1875  &  79.3  &  10.67  &  629  &  80.7 \\
    15  &  0.72  &  4749  &  70.9  &  2.66  &  1956  &  79.1  &  10.18  &  658  &  80.3 \\
    16  &  0.69  &  4992  &  70.5  &  2.53  &  2016  &  79.1  &   9.69  &  690  &  79.9 \\

  \bottomrule
  \end{tabular}
\end{table} 
% 68.626
