# Supplementary material for: Multi-criteria Token Fusion with One-step-ahead Attention for Efficient Vision Transformers
Source: arXiv:2403.10030 source file (2024-04-01)
Supplement: Supplementary file 8 [file table_s3.tex]

\begin{table}[h]
  \centering 
  \caption{\textbf{MCTF with other pretrained ViTs.}}
  \label{tab:sup3} 
  \setlength{\tabcolsep}{8pt}
  \begin{tabular}{c|cccc|cccc}
  
  \toprule
  % \multicolumn{1}{c|}{\multirow{3}{*}{$r$}}  &\multicolumn{3}{c|}{Deit-T}&  \multicolumn{2}{c}{Deit-B}\\
 $r$ & Models & FLOPs & thr. & acc. & Models & FLOPs & thr. & acc. \\
  \midrule
  %DeiT-T~\cite{touvron2021training}      &      &    3181  & 72.2      \\ 
     \rowcolor{gray} - & ViT-Ti & 1.26 & 3386 & 75.5 & ViT-S  &  4.61  &  1265  &  81.4 \\
     % 0  & ViT-Ti &  1.26 &  3386  &  75.5  & ViT-S & 4.61 &  1265  &  81.4 \\
     1  & ViT-Ti &  1.24 &  2884  &  75.4  & ViT-S & 4.51 &  1154  &  81.4 \\
     2  & ViT-Ti &  1.20 &  2964  &  75.4  & ViT-S & 4.38 &  1187  &  81.4 \\
     % 3  & ViT-Ti &  1.16 &  3059  &  75.4  & ViT-S & 4.24 &  1225  &  81.3 \\
     4  & ViT-Ti &  1.12 &  3151  &  75.3  & ViT-S & 4.10 &  1263  &  81.3 \\
     % 5  & ViT-Ti &  1.08 &  3254  &  75.3  & ViT-S & 3.97 &  1304  &  81.2 \\
     % 6  & ViT-Ti &  1.05 &  3362  &  75.3  & ViT-S & 3.83 &  1348  &  81.1 \\
     % 7  & ViT-Ti &  1.01 &  3510  &  75.1  & ViT-S & 3.70 &  1406  &  81.0 \\
     8  & ViT-Ti &  0.97 &  3651  &  75.2  & ViT-S & 3.56 &  1460  &  81.0 \\
     % 9  & ViT-Ti &  0.93 &  3796  &  75.0  & ViT-S & 3.43 &  1521  &  80.9 \\
    % 10  & ViT-Ti &  0.90 &  3958  &  75.1  & ViT-S & 3.30 &  1578  &  80.9 \\
    % 11  & ViT-Ti &  0.86 &  4110  &  74.9  & ViT-S & 3.17 &  1641  &  80.7 \\
    12  & ViT-Ti &  0.83 &  4288  &  74.7  & ViT-S & 3.04 &  1711  &  80.5 \\
    % 13  & ViT-Ti &  0.79 &  4469  &  74.3  & ViT-S & 2.91 &  1784  &  80.3 \\
    % 14  & ViT-Ti &  0.76 &  4660  &  74.2  & ViT-S & 2.79 &  1866  &  80.1 \\
    % 15  & ViT-Ti &  0.72 &  4869  &  73.8  & ViT-S & 2.66 &  1946  &  79.7 \\
    16  & ViT-Ti &  0.69 &  5073  &  73.3  & ViT-S & 2.53 &  2039  &  79.2 \\

     \multicolumn{1}{c}{}\\
  \toprule
 $r$ & Models & FLOPs & thr. & acc. & Models & FLOPs & thr. & acc. \\
  \midrule
  %DeiT-T~\cite{touvron2021training}      &      &    3181  & 72.2      \\ 
     \rowcolor{gray} - & ViT-B & 17.58 & 410 & 84.5 & ViT-L & 61.60 & 125 & 85.7 \\
      % 0  & ViT-B & 17.58  &  410  &  84.5  & ViT-L &  61.60  &  125  &  85.8  \\
      1  & ViT-B & 17.16  &  393  &  84.5  & ViT-L &  58.13  &  124  &  85.7  \\
      2  & ViT-B & 16.65  &  405  &  84.5  & ViT-L &  54.43  &  134  &  85.7  \\
      % 3  & ViT-B & 16.14  &  418  &  84.4  & ViT-L &  50.75  &       &        \\
      4  & ViT-B & 15.64  &  431  &  84.4  & ViT-L &  47.10  &  154  &  85.6  \\
      % 5  & ViT-B & 15.13  &  444  &  84.3  & ViT-L &  43.46  &       &        \\
      % 6  & ViT-B & 14.63  &  460  &  84.2  & ViT-L &  39.84  &       &        \\
      % 7  & ViT-B & 14.13  &  479  &  84.2  & ViT-L &  36.25  &       &        \\
      8  & ViT-B & 13.63  &  497  &  84.1  & ViT-L &  32.67  &  223  &  84.7  \\
      % 9  & ViT-B & 13.13  &  516  &  84.1  & ViT-L &         &       &        \\
     % 10  & ViT-B & 12.63  &  538  &  83.9  & ViT-L &         &       &        \\
     % 11  & ViT-B & 12.14  &  560  &  83.8  & ViT-L &         &       &        \\
     12  & ViT-B & 11.65  &  582  &  83.6  & \multicolumn{4}{c}{-}  \\
     % 13  & ViT-B & 11.16  &  607  &  83.5  & ViT-L &         &       &        \\
     % 14  & ViT-B & 10.67  &  636  &  83.2  & ViT-L &         &       &        \\
     % 15  & ViT-B & 10.18  &  666  &  82.8  & ViT-L &         &       &        \\
     16  & ViT-B &  9.69  &  698  &  82.3  & \multicolumn{4}{c}{-} \\

  %\bottomrule
  \multicolumn{1}{c}{}\\

  %\bottomrule
  \multicolumn{1}{c}{}\\

  \end{tabular}
\end{table} 
% 68.626
