# Supplementary material for: Multi-criteria Token Fusion with One-step-ahead Attention for Efficient Vision Transformers
Source: arXiv:2403.10030 source file (2024-04-01)
Supplement: Supplementary file 9 [file table_s4.tex]

\begin{table}[h]
  \centering 
  \caption{\textbf{Sensitivity analysis on the hyper-parameters.}}
  \label{tab:sup4} 
  \setlength{\tabcolsep}{8pt}
  \begin{tabular}{c|ccccccc}
  
  \toprule
  $\tau_\mathbf{a}$  &   1  &  1/2 &  1/5 & 1/10 &       1/25             & 1/100 \\
  \midrule
  acc.             & 79.1 & 79.4 & 79.7 & 79.7 &  \cellcolor{gray} 79.9 & 79.8  \\
  \bottomrule
  \multicolumn{1}{c}{}\\
  \toprule
  $\tau_\mathbf{s}$  &   1  & 1/2  & 1/5 & 1/10 & 1/25 & 1/100 \\
  \midrule
  acc.            & 79.6 & 79.7 & 79.8 & \cellcolor{gray} 79.9 & 79.8 & 79.8 \\
  \bottomrule
  \multicolumn{1}{c}{}\\
  \toprule
  $\alpha$           &  0.1 &  0.5 & 1 & 2 & 5 & 10 \\
  \midrule
  acc.          & 79.6 &  79.7 & \cellcolor{gray} 79.9 & 79.8 & 79.7 & 79.5 &  \\
  \bottomrule
  
  \end{tabular}
\end{table}
